# Supplementary material for: Non-equilibrium attractor for non-linear stochastic dynamics
Source: arXiv:2307.04728 ancillary file (2024-02-03)
Supplement: Supplementary file 1 [file PSTyP22-suppl-arXiv.pdf]

# Supplemental Material for "Non-equilibrium attractor for non-linear stochastic dynamics"

A. Patrón,[1,*] B. Sánchez-Rey,[2,†] E. Trizac,[3] and A. Prados[1,‡]

[1]*Física Teórica, Universidad de Sevilla, Apartado de Correos 1065, E-41080 Sevilla, Spain*
[2]*Departamento de Física Aplicada I, E.P.S., Universidad de Sevilla, Virgen de África 7, E-41011 Sevilla, Spain*
[3]*LPTMS, Université Paris-Saclay, CNRS, 91405, Orsay, France*

(Dated: July 10, 2023)

The analysis developed in this supplemental material provides insights on the general principles behind the emergence of the long-lived non-equilibrium state (LLNES). In Section I, we analyse the LLNES for a general isotropic algebraic potential. First, by going to Fourier space, we prove that the solutions of the noiseless Langevin equation tend to the LLNES, characterised by a Dirac-delta probability distribution function (pdf), in the long-time limit. Second, we analyse how the pdf evolves towards this form, by looking at its scaling properties—in particular, at its variance. Finally, we show how the LLNES emerges in the Fokker-Planck description, over an intermediate timescale. Also, by constructing a Lyapunov functional, it is shown that all the solutions of the Fokker-Planck equation tend to the LLNES over the same timescale. In Section II, we investigate the LLNES in more complex physical scenarios than those considered in the main text, mainly by a combination of intuitive arguments and numerical evidence. The analysed situations involve multiple-well potentials, anisotropy, and interactions for systems with more than one degree of freedom. We also give more details about the non-linear fluid considered in the main text, described at the kinetic level of description by the Boltzmann-Fokker-Planck equation—thus including binary collisions.

## I. EXTENDED ANALYSIS OF THE LLNES FOR ISOTROPIC SYSTEMS

In the main text, we have analysed an overdamped Brownian particle trapped in a $d$-dimensional non-linear potential with radial symmetry. Here, for the sake of concreteness and mathematical simplicity, we consider the family of algebraic potentials

$$U(r) = \frac{1}{n+1} k\, r^{n+1}, \quad n > 1. \tag{I.1}$$

The noiseless Langevin equation for this family of potentials is

$$\dot{r} = -br^n, \quad b \equiv k/\gamma, \quad r_i \equiv r(t=0) \implies (n-1)bt = r^{1-n}(t) - r_i^{1-n}. \tag{I.2}$$

The first (second) term is related to the time needed to relax from $r = +\infty$ to the instantaneous (initial) position $r(t)$ ($r_i$). For long enough times, we have that $r(t) \ll r_i$ and the second term becomes negligible against the first,

$$r(t) \to r_{\rm L}(t) \equiv [(n-1)bt]^{-\frac{1}{n-1}}, \quad r(t) \ll r_i. \tag{I.3}$$

In the main text, an analogous intuitive line of arguments led us to conclude—not rigorously from a mathematical point of view—that the pdf tends to the delta, i.e. $P(r,t) \to \delta(r - r_{\rm L}(t))$, i.e., that the average value of any function of $r$, $\langle \chi(r) \rangle$, tends to $\chi(r_{\rm L}(t))$.This is non-rigorous since, for any time $t$, there is a range of values of $r_i$ close to zero such that $r_i$ is of the order of $r_{\rm L}(t)$ or smaller, and thus one cannot ensure that $\langle \chi(r) \rangle \to \chi(r_{\rm L}(t))$ for an arbitrary function $\chi$.

Next, we present rigorous arguments for the emergence of the LLNES in the radial symmetry case after a deep quench. First, still within the framework of the noiseless Langevin (or deterministic) equation, we show that the above intuitive line of arguments can be formalised in a more rigorous way. In Sec. I A, we prove that the Fourier transform of $P(r,t)$ converges to the Fourier transform of the Dirac-delta, which shows their being equivalent to calculate the average of arbitrary functions of $r$. In Sec. I B, we further analyse the scaling behaviour of the distribution $P(r,t)$ to discern how it tends to the Dirac-delta peak, paying special attention to the tails of the distribution. Second,

* apatron@us.es
† bernardo@us.es
‡ prados@us.es

in Sec. I C, we consider the complete Fokker-Planck equation to show that inclusion of noise does not destroy the emergence of the LLNES, but only restricts it to an intermediate timescale. This is done in two complementary ways. In Sec. I C 1, the LLNES is derived as an asymptotic solution of the Fokker-Planck equation over an intermediate timescale—which exists if the system has been submitted to a deep quench, i.e. if $T_f \ll T_i$. In Sec. I C 2, we build a Lyapunov functional to prove that the LLNES—i.e. the asymptotic solution derived in Sec. I C 1—is monotonically approached by all the solutions of the Fokker-Planck equation over the same timescale.

### A. Fourier transform of $P(r,t)$

Here, we prove that the Fourier transform of $P(r,t)$ converges to the Fourier transform of the Dira-delta peak in the long-time limit. We start from explictly rewriting $r(t)$ from Eq. (I.2) as

$$r(t) = f(r_i,t) \equiv r_i \left[1 + (r_i/r_{\mathrm{L}}(t))^{n-1}\right]^{-\frac{1}{n-1}}. \tag{I.4}$$

If $P_i(r_i)$ is the initial pdf for the initial conditions $r_i$, then the pdf $P(r,t)$ of $r$ at any time $t$ is

$$P(r,t) = \int_0^{+\infty} dr_i\, \delta\left(r - f(r_i,t)\right) P_i(r_i), \tag{I.5}$$

Note that $P(r,t) = 0$ for $r > r_{\mathrm{L}}(t)$, because $f(r_i,t) \le r_{\mathrm{L}}(t)$ for the algebraic family we are considering. The argument for the emergence of the Dirac-delta above—and in the main text—is equivalent to substitute $f(r_i,t)$ with $r_{\mathrm{L}}(t)$ in Eq. (I.5) by considering that $r_{\mathrm{L}}(t) \ll r_i$: this is non-rigorous since, for any time $t$, there is a range of values of $r_i$ close to zero such that $r_i$ is of the order of $r_{\mathrm{L}}(t)$ or smaller.

In order to proceed, it is useful to go to Fourier space by introducing the characteristic function

$$G(k,t) \equiv \left\langle e^{ikr}\right\rangle = \int_0^{\infty} dr\, e^{ikr} P(r,t) = \int_0^{\infty} dr_i\, e^{ikf(r_i,t)} P_i(r_i). \tag{I.6}$$

Now we consider the long-time limit. We split the integration over $r_i$ into two slices: from 0 to $\varepsilon(t)$, and from $\varepsilon(t)$ to $+\infty$. We choose $\varepsilon(t)$ small, in the sense that $\varepsilon(t) \to 0$ in the limit as $t \to \infty$ but such that $\varepsilon(t)/r_{\mathrm{L}}(t) \gg 1$. Therefore, in the second slice we can safely substitute $f(r_i,t)$ with $r_{\mathrm{L}}(t)$, with an error that goes to zero for long times:

$$\begin{aligned} G(k,t) &= \int_0^{\varepsilon(t)} dr_i e^{ikf(r_i,t)} P_i(r_i) + \int_{\varepsilon(t)}^{\infty} dr_i e^{ikf(r_i,t)} P_i(r_i) \sim \int_0^{\varepsilon(t)} dr_i e^{ikf(r_i,t)} P_i(r_i) + e^{ikr_{\mathrm{L}}(t)} \int_{\varepsilon(t)}^{\infty} dr_i P_i(r_i) \\ &= e^{ikr_{\mathrm{L}}(t)} + \underbrace{\int_0^{\varepsilon(t)} dr_i \left(e^{ikf(r_i,t)} - 1\right) P_i(r_i)}_{\Delta G(k,t)}, \quad t \to +\infty. \end{aligned} \tag{I.7}$$

The first term is the Fourier transform of the Dirac-delta, the second term $\Delta G(k,t)$ can be shown to go to zero:

$$|\Delta G(k,t)| = \left| \int_0^{\varepsilon(t)} dr_i \left(e^{ikf(r_i,t)} - 1\right) P_i(r_i) \right| \le \int_0^{\varepsilon(t)} dr_i \left| e^{ikf(r_i,t)} - 1 \right| P_i(r_i) \le 2 \int_0^{\varepsilon(t)} dr_i P_i(r_i) \to 0, \quad t \to +\infty. \tag{I.8}$$

In conclusion, we have rigorously proved that

$$G(k,t) \sim e^{ikr_{\mathrm{L}}(t)}, \quad t \to +\infty \iff P(r,t) \sim \delta\left(r - r_{\mathrm{L}}(t)\right), \quad t \to +\infty. \tag{I.9}$$

In this formal proof, we would like to emphasise that (i) we have not employed the explicit form of $f(r_i,t)$ in Eq. (I.4), but only that $f(r_i,t)$ "forgets" the initial condition $r_i$ in the long-time limit, and (ii) the shape of the pdf for the initial conditions $P_i(r_i)$ is completely general.

### B. Scaling behaviour and tails of the distribution

Now we look into the structure of the pdf $P(r,t)$ in more detail. Specifically, we would like to investigate how $P(r,t)$ tends to the $P_{\mathrm{L}}(r,t)$, by analysing its scaling behaviour when converging towards the Dirac-delta solution.

With this aim, it is convenient to introduce the "length" [1] scale $\ell_i$ associated with the initial conditions: for the usual equilibrium initial conditions, we have that

$$\ell_i \equiv (\beta_i k)^{-\frac{1}{n+1}} = (k_B T_i/k)^{\frac{1}{n+1}}. \tag{I.10}$$

In general, we consider that

$$P_i(r_i) = \ell_i^{-1} P_i^*(r_i^* = r_i/\ell_i), \quad r_i^* = r_i/\ell_i, \tag{I.11}$$

where $P_i^*$ is an arbitrary (non-negative) function—the pdf of the dimensionless variable $r_i^*$. Accordingly, $P(r,t) = \ell_i^{-1} P^*(r^*,t)$, $r^* = r/\ell_i$.

Since $r^*$ is very close to $r_{\rm L}^*(t)$ for long times, we assume that the deviations of $r^*$ from $r_{\rm L}^*(t)$ are small and scale as some power of $r_{\rm L}^*(t)$. We thus define a new variable $\xi$, of the order of unity, with pdf $\phi(\xi,t)$ as follows:

$$r^* \equiv r_{\rm L}^*(t) + \xi\, [r_{\rm L}^*(t)]^{\psi} \quad \text{or} \quad \xi = (r^* - r_{\rm L}^*(t)) \,/\, [r_{\rm L}^*(t)]^{\psi} \implies \phi(\xi,t) = [r_{\rm L}^*(t)]^{\psi}\, P^*(r^*,t), \tag{I.12}$$

where $\psi > 0$ is a parameter to be determined later. Here we use the explicit form of $f(r_i,t)$ in Eq. (I.4) to write

$$\phi(\xi,t) = \frac{r_{\rm L}^*(t)^{\psi}}{\left[1 - \left(1 + \xi\, [r_{\rm L}^*(t)]^{\psi-1}\right)^{n-1}\right]^{\frac{n}{n-1}}} P_i^* \left( \frac{r_{\rm L}^*(t) + \xi r_{\rm L}^*(t)^{\psi}}{\left[1 - (1 + \xi r_{\rm L}^*(t)^{\psi-1})^{n-1}\right]^{\frac{1}{n-1}}} \right), \qquad -[r_{\rm L}^*(t)]^{1-\psi} \le \xi \le 0. \tag{I.13}$$

In the long-time limit, $r_{\rm L}^*(t) \to 0$, and as long as $|\xi|\, [r_{\rm L}^*(t)]^{\psi-1} \ll 1$, we can introduce the approximation

$$\left(1 + \xi\, [r_{\rm L}^*(t)]^{\psi-1}\right)^{n-1} = 1 + \xi(n-1)\, [r_{\rm L}^*(t)]^{\psi-1} + O(|\xi|\, [r_{\rm L}^*(t)]^{\psi-1})^2,$$

and then

$$\phi(\xi,t) \sim \frac{[r_{\rm L}^*(t)]^{\frac{n-\psi}{n-1}}}{[(n-1)(-\xi)]^{\frac{n}{n-1}}} P_i^* \left( \frac{[r_{\rm L}^*(t)]^{\frac{n-\psi}{n-1}}}{[(n-1)(-\xi)]^{\frac{1}{n-1}}} \right), \quad |\xi|\, [r_{\rm L}^*(t)]^{\psi-1} \ll 1. \tag{I.14}$$

This equation suggests that $\psi = n$: with this choice, $\phi(\xi,t)$ becomes time-independent and thus

$$\phi(\xi,t) \sim \phi_{\rm st}(\xi) \equiv [(n-1)(-\xi)]^{-\frac{n}{n-1}}\, P_i^* \left( [(n-1)(-\xi)]^{-\frac{1}{n-1}} \right), \quad |\xi|\, [r_{\rm L}^*(t)]^{n-1} \ll 1, \tag{I.15}$$

implying that $P^*(r^*,t) = [r_{\rm L}^*(t)]^{-n}\, \phi_{\rm st}\left((r^* - r_{\rm L}^*(t)) / [r_{\rm L}^*(t)]^n\right)$ presents scaling properties for long times.

Equation (I.15) measures the deviations from the Dirac-delta, which can be visualised as the left tails on the left panel in Fig.1 of the main text. Provided that $\phi_{\rm st}(\xi)$ has finite variance, the found scaling entails that the standard deviation of $r^*$, $\sigma^*_{r^*}(t)$, scales as $[r_{\rm L}^*(t)]^n$ for long times and thus $\sigma_{r^*}(t)/\langle r^* \rangle(t) \propto [r_{\rm L}^*(t)]^{n-1} \to 0$, which is a signature of the emergence of the Dirac-delta distribution [2]. It is interesting to compare the "width of the Dirac-delta", as measured by $\sigma^*_{r^*}(t)$, and the width of the final equilibrium distribution, which—in the dimensionless variables we are using here—is given by $\ell_f^* = \ell_f/\ell_i$, where $\ell_f$ is the characteristic width of the final distribution. Note that this is a relevant question: $\ell_f^*$ also tends to zero for a deep quench, since for a final equilibrium canonical distribution we have that $\ell_f = (\beta_f k)^{-\frac{1}{n+1}}$, i.e. $\ell_f^* = (\beta_f/\beta_i)^{-\frac{1}{n+1}} = (T_f/T_i)^{\frac{1}{n+1}} \to 0$. To ensure that the Dirac-delta is in fact much narrower than the final distribution we have to impose that $\sigma^*_{r^*}(t)/\ell_f^* \propto [r_{\rm L}^*(t)]^n/(T_f/T_i)^{\frac{1}{n+1}} \ll 1$, i.e.

$$[r_{\rm L}^*(t)]^n \ll (T_f/T_i)^{\frac{1}{n+1}}. \tag{I.16}$$

Note that $\phi_{\rm st}(\xi)$ depends on the details of the initial distribution. Yet, under quite general conditions, the scaling function $\phi_{\rm st}(\xi)$ presents universal features. To start with, we have that

$$\lim_{\xi \to -\infty} \phi_{\rm st}(\xi) = 0, \quad \lim_{\xi \to 0^-} \phi_{\rm st}(\xi) = 0. \tag{I.17}$$

The first condition follows as long as $P_i^*(r_i^*)$ remains finite or $P_i^*(r_i^*)$ diverges slower than $r_i^{*\,-n}$ for small $r_i^*$; the second condition follows as long as $P_i^*(r_i^*)$ does not have "fat" tails, i.e. when $P_i^*(r_i^*)$ decays faster than algebraic towards zero for large values of its argument. Equation (I.17) implies that $\phi_{\rm st}(\xi)$ presents a non-monotonic behaviour

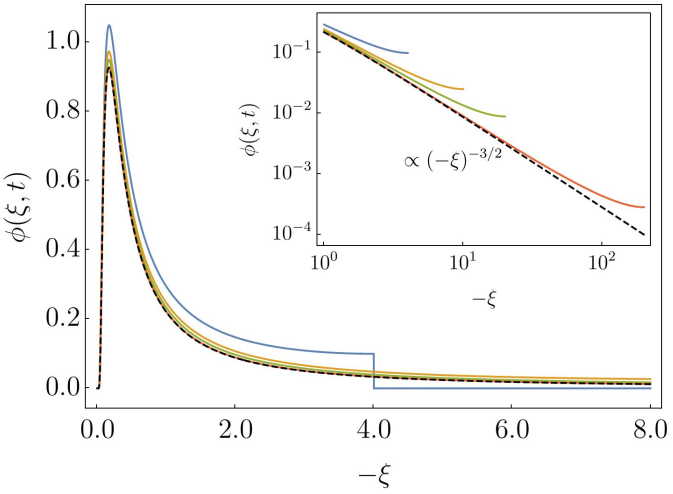


FIG. S1. Pdf for the scaled variable $\xi$ defined in Eq. (I.12). The data shown corresponds to the case $n = 3$, specifically we plot the curves obtained from Eq. (I.13) for different times $t = 2, 5, 10$ and 100 (full curves) together with the stationary distribution in Eq.(I.15) (black-dashed curve). The inset is displayed in logarithmic scale, such that the algebraic tails for large $\xi$ from Eq.(I.18) are visualised—the dashed straight line with slope $-3/2$.

with a maximum at intermediate values of $\xi$. Both the position and the height of such maximum depend on the details of the initial distribution $P_i^*(r_i^*)$. The large $\xi$ behaviour involves a power-law tail of the form

$$\phi_{\rm st}(\xi) \sim P_i^*(0)\,[(n-1)(-\xi)]^{-\frac{n}{n-1}} \propto (-\xi)^{-\frac{n}{n-1}}, \tag{I.18}$$

if $P_i^*(0) \neq 0$. This behaviour is universal, in the sense that it only depends on the potential acting on the Brownian particle (through $n$) while the initial conditions are completely encoded within the multiplicative constant.

Figure S1 shows the pdf for the scaled variable $\xi$. We observe how $\phi(\xi,t)$ approaches the steady solution $\phi_{\rm st}(\xi)$ as time increases. In the inset we employ a logarithmic scale to illustrate the tails of the distribution, as given by Eq. (I.18). Note that the pdf departs from the theoretical tail for very large values of $|\xi|$, with the separation point moving to higher values of $|\xi|$ as time increases. This is consistent with our theoretical analysis, since the steady distribution in Eq. (I.15) is valid only when $|\xi|\,[r_{\rm L}^*(t)]^{n-1} \ll 1$, i.e. we expect that it no longer describes $P^*(r^*,t)$ for $|\xi| = O(r_{\rm L}^*(t))^{-(n-1)}$.

### C. LLNES from the Fokker-Planck framework

Now, we show how the LLNES emerges in the Fokker-Planck description, including the noise. The main point is the existence of an intermediate timescale for systems submitted to a deep temperature quench, $T_f \ll T_i$, in which noise is subdominant. Over this timescale (i) we prove that the LLNES emerges as an asymptotic long-time solution of the Fokker-Planck equation, and (ii) we construct a Lyapunov functional to establish the global stability of the LLNES, i.e. that all the solutions of the Fokker-Planck equation tend thereto over the considered timescale.

#### 1. *LLNES as an asymptotic solution of the Fokker-Planck equation*

It is convenient to rescale $\boldsymbol{r}$ with a characteristic time-dependent "length" $\ell(t)$ and accordingly rescale the pdf. For the sake of simplicity, we choose

$$\ell(t) = \sqrt{\langle r^2\rangle(t)}, \quad \boldsymbol{c} \equiv \boldsymbol{r}/\ell(t), \quad \phi(\boldsymbol{c},t) = \ell^d(t) P(\boldsymbol{r},t). \tag{I.19}$$

From the Fokker-Planck equation, it is readily obtained that

$$\gamma \frac{d}{dt}\left\langle r^2\right\rangle(t) = -2\left[k\left\langle r^{n+1}\right\rangle(t) - d k_B T_f\right]. \tag{I.20}$$

At equilibrium, in agreement with the equipartition theorem, we have $k\left\langle r^{n+1}\right\rangle = dk_B T_f$, or $\left\langle r^{n+1}\right\rangle = d\,\ell_f^{n+1}$. The Fokker-Planck equation for the rescaled pdf, including the noise, is

$$\partial_t \phi = b\,\ell^{n-1}\nabla_{\boldsymbol{c}}\cdot\left\{\left[c^{n-1}-M_{n+1}\right]\boldsymbol{c}\,\phi+\frac{k_B T_f}{k\,\ell^{n+1}}\left[d\boldsymbol{c}\phi+\nabla_{\boldsymbol{c}}\phi\right]\right\}, \tag{I.21}$$

where $b$ was defined in Eq. (I.2), $M_n \equiv \langle c^n\rangle = \langle r^n\rangle/\ell^n$, and we have taken into account that, by definition, $M_2 = 1$.

It is convenient to employ here the dimensionless variables introduced in the previous section, specifically

$$\ell(t) = \ell_i \ell^*(t) = (k_B T/k)^{1/(n+1)}\ell^*(t), \qquad \ell^*\frac{d\ell^*(t)}{dt} = -b\,\ell_i^{n-1}\left(\ell^{*\,n+1}M_{n+1} - d\,T_f/T_i\right), \tag{I.22}$$

where $\ell^*(t)$ is of the order of unity for not very long times. Introducing the above relation into Eq. (I.21), we get

$$\partial_t \phi = b\,\ell_i^{n-1}\ell^{*\,n-1}\,\nabla_{\boldsymbol{c}}\cdot\left\{\left[c^{n-1}-M_{n+1}\right]\boldsymbol{c}\,\phi+\ell^{*\,-(n+1)}(T_f/T_i)\left[d\boldsymbol{c}\phi+\nabla_{\boldsymbol{c}}\phi\right]\right\}. \tag{I.23}$$

Now we define a new timescale $s$, such that

$$ds = b\,\ell_i^{n-1}\ell^{*\,n-1}dt \implies \partial_s\phi = \nabla_{\boldsymbol{c}}\cdot\left\{\left[c^{n-1}-M_{n+1}\right]\boldsymbol{c}\,\phi+\ell^{*\,-(n+1)}(T_f/T_i)\left[d\boldsymbol{c}\phi+\nabla_{\boldsymbol{c}}\phi\right]\right\}. \tag{I.24}$$

Equation (I.24) is exact, and thus valid for any temperature ratio $T_f/T_i$. Notwithstanding, since we are interested in a quench from a high temperature, we have that $T_i \gg T_f$ and the last term on the rhs of Eq. (I.24) is subdominant and can be neglected—as long as $\ell^{*\,-(n+1)}T_f/T_i \ll 1$. Then we have

$$\partial_s\phi \sim \nabla_{\boldsymbol{c}}\cdot\left\{\left[c^{n-1}-M_{n+1}\right]\boldsymbol{c}\,\phi\right\}, \quad \ell^{*\,-(n+1)}T_f/T_i \ll 1. \tag{I.25}$$

Note that the initial condition—equilibrium at temperature $T_i$—has radial symmetry and the time evolution preserves it, and thus $\phi(\boldsymbol{c},t)$ will also have radial symmetry at all times. Equation (I.25) admits a stationary solution $\phi_{\text{st}}(\boldsymbol{c})$ with radial symmetry, $\phi_{\text{st}}(\boldsymbol{c}) = \Omega_d^{-1}\phi_{\text{st}}(c)$—where $\Omega_d$ is the $d$-dimensional solid angle:

$$\nabla_{\boldsymbol{c}}\cdot\left\{\left[c^{n-1}-M_{n+1}\right]\boldsymbol{c}\,\phi_{\text{st}}(c)\right\} = 0 \iff \left[c^{n-1}-M_{n+1}\right]\phi_{\text{st}}(c) = 0, \tag{I.26}$$

The above equality for $\phi_{\text{st}}$ is readily translated to an infinite hierarchy for the moments $M_m$, $m = 0,1,2,\ldots$,

$$0 = \int d\boldsymbol{c}\,c^m\left[c^{n-1}-M_{n+1}\right]\phi_{\text{st}}(\boldsymbol{c}) = \int_0^\infty dc\,c^{d-1}\,c^m\left[c^{n-1}-M_{n+1}\right]\phi_{\text{st}}(c) = M_{m+n-1} - M_m M_{n+1}, \quad M_0 = 1. \tag{I.27}$$

The particular case $m = 2$ implies that $M_2 = 1$, in agreement with the definition of scaled variables in Eq. (I.19).

Equation (I.27) entails that

$$M_m = 1,\ \forall m > 0, \implies \phi_{\text{st}}(c) = \phi_{\text{L}}(c) \equiv \delta(c-1), \iff \phi_{\text{st}}(\boldsymbol{c}) = \phi_{\text{L}}(\boldsymbol{c}) = \Omega_d^{-1}\phi_{\text{L}}(c), \tag{I.28}$$

i.e. $\phi_{\text{st}}$ corresponds to the LLNES. In turn, $\langle r\rangle(t) = \ell(t)M_1(t) = \ell(t) = r_{\text{L}}(t)$, with $r_{\text{L}}(t)$ as given by Eq. (I.3): making use of Eq. (I.22), $\ell(t)$ evolves in accordance with the noiseless equation (I.2),

$$\dot{\ell}^* = -b\,\ell_i^{n-1}\ell^{*\,n} \iff \dot{\ell} = -b\,\ell^n, \quad \ell^{*\,-(n+1)}T_f/T_i \ll 1. \tag{I.29}$$

This is consistent with our approach in the main text and in the previous section, which disregards the noise in the Langevin equation, provided that $t$ is not too long. Note the complete analogy with Eq. (I.2), but the more complete analysis developed here has allowed us to identify the intermediate timescale over which the LLNES is developed, $\ell^{*\,-(n+1)}T_f/T_i \ll 1$. The larger the temperature ratio $T_i/T_f$ is, the wider this intermediate timescale—and the more relevant the LLNES—becomes.

### 2. *Global stability of the LLNES: Lyapunov functional and H-theorem*

Now we prove that all the solutions of the Fokker-Planck equation, over the intermediate timescale $\ell^{*\,-(n+1)}T_f/T_i \ll 1$ we have just found, approach the LLNES. With this aim, we introduce the following $H$-functional

$$H(t) \equiv -\langle \ln c\rangle = -\int d\boldsymbol{c}\ \phi(\boldsymbol{c},t)\ln c, \tag{I.30}$$

which we show below to be a Lyapunov functional. Employing Jensen's inequality, it is readily seen that $H$ is bounded from below by its global minimum, $H(t) = -\left\langle \ln(c^2) \right\rangle /2 \geq -\ln\left\langle c^2 \right\rangle /2 = -\ln M_2/2 = 0$, which is attained at the LLNES: $H_\text{L} = -\int d\boldsymbol{c}\, \phi_\text{L}(\boldsymbol{c}) \ln c = -\int_0^{+\infty} dc\, c^{d-1}\, \delta(c-1) \ln c = 0$.

Now we consider the time evolution of $H(t)$. It is convenient to employ the timescale $s$ defined in Eq. (I.24),

$$\frac{dH}{ds} = -\int d\boldsymbol{c}\, \partial_s \phi \ln c = \int d\boldsymbol{c}\, \left\{ \left[ c^{n-1} - M_{n+1} \right] \boldsymbol{c}\, \phi + \ell^{*-(n+1)} (T_f/T_i) \left[ d\boldsymbol{c}\phi + \nabla_{\boldsymbol{c}} \phi \right] \right\} \cdot \nabla_{\boldsymbol{c}} \ln(c) \tag{I.31}$$

where we have employed Eq. (I.24) and integrated by parts, assuming that the boundary term vanishes at infinity. Once again, in the limit $T_i \gg T_f$, the term proportional to $\nabla_{\boldsymbol{c}} \phi$ can be neglected as long as $\ell^{*-(n+1)}(T_f/T_i) \ll 1$, which we will comment on later. Therefore,

$$\frac{dH}{ds} \sim \int d\boldsymbol{c}\, \left[ c^{n-1} - M_{n+1} \right] \phi\; \boldsymbol{c} \cdot \nabla_{\boldsymbol{c}} \ln c = \int d\boldsymbol{c}\, \left[ c^{n-1} - M_{n+1} \right] \phi = M_{n-1} - M_{n+1} \leq 0, \quad \ell^{*-(n+1)}(T_f/T_i) \ll 1, \tag{I.32}$$

where we have used that $\boldsymbol{c} \cdot \nabla_{\boldsymbol{c}} \ln c = 1$. The equality holds at the LLNES, for which $M_m = 1\ \forall m$. For the very last step of the proof, we have made use of $M_r \geq (M_s)^{r/s}$ for $r > s > 0$, which stems from Hölder's inequality [3]:

$$M_{n-1} - M_{n+1} \leq M_{n+1}^{\frac{n-1}{n+1}} - M_{n+1} = M_{n+1}^{\frac{n-1}{n+1}} \left( 1 - M_{n+1}^{\frac{2}{n+1}} \right) \leq M_{n+1}^{\frac{n-1}{n+1}} \left( 1 - M_2 \right) = 0, \tag{I.33}$$

where we have brought to bear that $n > 1$ and $M_2 = 1$.

Since $H$ is a non-increasing function of time bounded from below, $H$ tends to a well-defined limit for $s \gg 1$ at which $dH/ds$ vanishes: therefore, $H$ is a Lyapunov functional over the timescale $s$ and all solutions of the Fokker-Planck equation tend thereto over this timescale. It must be stressed that this H-theorem holds exclusively within the timescale $s$, and ceases to be valid when $\ell^{*-(n+1)}(t)(T_f/T_i)$ becomes of the order of unity. This comes about when $\ell^*$ becomes close to its equilibrium value at $T_f$: when $\ell^*(t) = O(\ell^*_\text{eq}(T_f))$, we have that $\ell^*(t) = O((T_f/T_i)^{1/(n+1)})$, recalling the definition of $\ell^*(t)$, as given by Eq. (I.22). In other words, the LLNES disappears when $\langle r \rangle (t)$ becomes of the order of the equilibrium value at the final temperature $T_f$, as stated on physical grounds in the main text.

Therefore, we have rigorously proven that the LLNES "attracts" all the solutions of the Fokker-Planck equation over the intermediate time scale for which $s \gg 1$ and noise is negligible, i.e. $\ell^{*-(n+1)} T_f/T_i \ll 1$. Note that this condition is compatible with that for the Dirac-delta being actually narrower than the final equilibrium distribution in Eq. (I.16), we can unify both of them as $(T_f/T_i)^{\frac{1}{n+1}} \ll r^*_\text{L}(t) \ll (T_f/T_i)^{\frac{1}{n(n+1)}}$.

## II. ROBUSTNESS OF THE LLNES IN MORE COMPLEX SCENARIOS

In the main text and up to now, we have focused our study of the LLNES on isotropic situations, to illustrate its main features in a way that allows for analytical computations and rigorous—from a physics perspective—proofs. Here, we give reasons, mainly by the combination of intuitive arguments and results, both analytical and numerical, in some specific, simple, cases, that the LLNES may extend to a wider variety of scenarios.

In order to illustrate and support these insights, we analyse below different relevant physical potentials in which the LLNES comes about: with multiple minima, anisotropy, and interacting degrees of freedom. We also elaborate on the case of the interacting system considered in the main text: a fluid of $N$ particles with non-linear drag force and binary (possibly inelastic) collisions, for which our framework still applies—although the starting point does not correspond to the non-linear Langevin equation employed in the remainder of this work.

### A. Intuitive picture for the emergence of the LLNES

Let us consider a $d$-dimensional overdamped system trapped in a general confining potential $U(\boldsymbol{r}) = U(x_1, x_2, ..., x_d)$. For instance, that would be the case of an overdamped Brownian particle confined in an optical trap, for which $\boldsymbol{r}$ would account for its cartesian coordinates, or the case of a molecular fluid with non-linear drag at the kinetic level, where $\boldsymbol{r}$ here would instead stand for the single-particle velocities, and the corresponding "confining potential" would be the velocity-dependent function whose gradient in velocity space provides the non-linear drag force—see Sec. II E. In any case, such general potential may have a plethora of minima due to either the form of the external force or as a result of the repulsive interactions between the different degrees of freedom. Such minima define different characteristic lengths

(i.e. the positions of those minima with respect to the origin) that, as long as the initial temperature is sufficiently high, become irrelevant for the dynamics of concern—as argued below.

Giving a rigorous condition for the emergence of the LLNES in such a general situation is a challenging mathematical problem, which lies outside the scope of the present work. Yet, one can get an intuition about the conditions under which the LLNES emerges by analysing some specific examples, both analytically—when their simplicity makes it possible—and numerically. This is the approach that we follow in the remainder of this section, in which we consider several relevant examples to illustrate some common features appearing in all of them.

We stress that the general picture drawn in the following paragraphs anticipates the common features behind the LLNES in the different examples we investigate afterwards, which hint at—but not prove—the existence of a general framework for it. The emergence and shape of the LLNES seem to be related to the dominant contributions of $U(\boldsymbol{r})$ for large $r$, which we refer to as the effective potential $U_{\text{eff}}(\boldsymbol{r})$ in the following. The effective potential $U_{\text{eff}}(\boldsymbol{r})$ corresponds to the potential that the system feels initially, since the initial condition corresponds to a high temperature and thus the details of the bottom of the potential $U(\boldsymbol{r})$ are irrelevant. Our analysis of the isotropic case suggests that it is the necessary that the force diverges faster than linearly at large distances, more specifically that $\lim_{r\to\infty} |\boldsymbol{A}(\boldsymbol{r})|/r \to \infty$.

The main intuitive idea stems from the stream plots of the effective force $-\nabla U_{\text{eff}}(\boldsymbol{r})$—see Fig. S3. In the deterministic dynamics, the movement of the particle follows the stream lines, since $\dot{\boldsymbol{r}} \propto -\nabla U_{\text{eff}}(\boldsymbol{r})$ and thus the probability weight tends to accumulate along the directions in which the force exerted on the system increases the slowest. A graphical image may be given by imagining a "snowplough" acting on the directions of the fastest variation of the force, and thus concentrating the probability weight over the slowest ones. For long enough times, the analysis of the specific cases considered below suggests that, regardless of the initial probability—or snow—distribution, all the probability accumulates over the slowest directions, the initial conditions become immaterial, and the Dirac-delta pdf characterising the LLNES emerges for faster-than-linearly diverging forces.

We would like to highlight that the symmetries of the confining potential have an impact on the geometrical structure of the LLNES. In this context, symmetries refer to the presence of cyclic variables in the potential $U(\boldsymbol{r})$, when expressed in a certain coordinate system. In the main text and in Sec. I of this supplemental material, we have analysed in depth the radially symmetric (or isotropic) situation, where $U$ only depends on the distance to the origin $r$ and the $d$-dimensional solid-angle variables are thus cyclic. That analysis shows that the LLNES has also radial symmetry in this case and, on a physical basis, one expects that this will also be the case for other symmetries. Anyway, rigorously characterising the geometrical structure of the LLNES for a completely general situation is a non-trivial task, which is worth investigating in future work.

### B. Potentials with multiple minima

In the main text, we briefly analysed the case of an overdamped Brownian particle confined in a multistable "lemon-squeezer" potential, i.e. the potential in Eq. (13) with $k < 0$. For the $d$-dimensional case, there is a continuous set of minima over the hyper-surface $r = r_c \equiv \sqrt{|k|/\lambda}$; two minima at $x = \pm r_c$ for $d = 1$. The corresponding noiseless Langevin equation is

$$\dot{r} = ar - br^3, \; a \equiv k/\gamma, \, b \equiv \lambda/\gamma \implies r(t) = r_i \, e^{at} \left[1 + (r_i^2/r_c^2)\left(e^{2at} - 1\right)\right]^{-1/2}, \tag{II.1}$$

we recall that $r_i \equiv r(t=0)$. Logically, $\lim_{t\to\infty} r(t) = r_c = \sqrt{|a|/b} = \sqrt{|k|/\lambda}$; $r_c$ corresponds to mechanical stability.

In the main text, we showed that the LLNES for $k < 0$ emerges in a completely similar way as that for $k > 0$. Here, we also employ dimensionless temperature as in the main text, $T^* = k_B T \lambda/k^2$. Provided that $T_i^* \gg 1$, there appears an intermediate time window such that $r_i \gg r(t) \gg r_c$, over which

$$r(t) \sim (2bt)^{-1/2} = r_{\text{L}}(t), \quad 1 \gg 2at \gg r_c^2/r_i^2. \tag{II.2}$$

We stress that $r_{\text{L}}(t)$ in Eq. (II.2) is identical to that of Eq. (16) in the main text for $k > 0$, since it only depends on the "effective potential" $U_{\text{eff}}(r) = \lambda r^4/4$ at large distances. A relevant question is whether the LLNES extends to longer times for low enough final temperatures $T_f^* \ll 1$, similarly to the case $k > 0$. The answer is positive: if $r_i \gg r_c$ and $2at = O(1)$, Eq. (II.1) gives $r(t) \sim r_{\text{L}}(t) = r_c \left(1 - e^{-2at}\right)^{-1/2}$. The system follows the deterministic evolution towards mechanical equilibrium at $r = r_c$, with small thermal fluctuations—as observed in Fig. S2.

In other words, the presence of multiple minima only induces additional characteristic lengths, corresponding to "mechanical equilibrium", which have to be taken into account. Nevertheless, as long as we initially have a sufficiently high temperature, the system forgets its initial conditions while moving under the action of the "effective potential" felt at large distances and falls on a LLNES regime that is independent of these new lengths. If the final temperature is low enough, the LLNES extends to longer times and the system approaches over it mechanical equilibrium, with small thermal fluctuations around it.

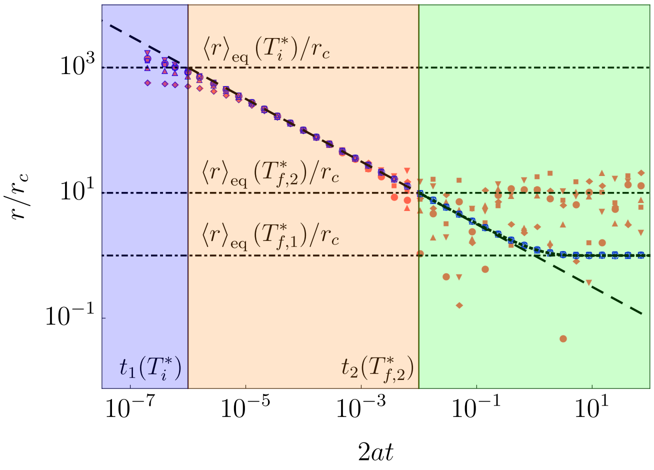


FIG. S2. Stochastic trajectories for an overdamped Brownian particle trapped in a non-linear potential given by Eq.(13) with $k < 0$. The initial and final equilibrium temperatures and the colour codes are the same as those presented in Fig. 1 from the main text. The diagonal dashed line corresponds to the LLNES in Eq. (II.2)—or Eq. (16) of the main text, which is thus valid for both signs of $k$.

### C. Anisotropic potentials

So far, our discussion has been focused on overdamped systems with radial symmetry, in which the relevant dynamics is given by the radial coordinate $r \equiv |\boldsymbol{r}| = \sqrt{x_1^2 + x_2^2 ... + x_d^2}$. Here, we show that such a restriction is not necessary for the emergence of the LLNES, by considering some specific examples.

As a first example, let us consider a two-dimensional confining potential of the form

$$U(x_1, x_2) = \left(k_1 x_1^4 + k_2 x_2^4\right)/4, \quad k_1, k_2 > 0, \tag{II.3}$$

which gives the following set of decoupled noiseless Langevin equations:

$$\dot{x}_i = -b_i x_i^3, \quad b_i \equiv k_i/\gamma,\, i = 1, 2 \implies x_i(t) = x_{i,0}\left(1 + 2x_{i,0}^2 b_i t\right)^{-1/2} \xrightarrow{\text{long } t} \pm\, x_{i,\rm L}(t) \equiv \pm\, (2b_i t)^{-1/2}. \tag{II.4}$$

In the above, $x_{j,i}$ is the initial value of $x_j(t)$, and the $\pm$ sign stems from that of $x_{j,0}$. The two coordinates, $x_1$ and $x_2$ tend independently to their respective LLNES, $\left[\delta(x_i - x_{i,\rm L}) + \delta(x_i + x_{i,\rm L})\right]/2$, which means that

$$P_{\rm L}(x_1, x_2; t) = \frac{1}{4}\left[\delta(x_1 - x_{1,\rm L}(t)) + \delta(x_1 + x_{1,\rm L}(t))\right]\left[\delta(x_2 - x_{2,\rm L}(t)) + \delta(x_2 + x_{2,\rm L}(t))\right]. \tag{II.5}$$

The above solution holds regardless of the values of $b_1$ and $b_2$, i.e. of $k_1$ and $k_2$. However, these constants define two different timescales ($\tau_1 \propto b_1^{-1}$ and $\tau_2 \propto b_2^{-1}$, respectively) that must be taken into account to discern whether the system has reached the LLNES or not. For instance, in the extreme case where $b_1 \gg b_2$, by the time that $x_1(t)$ reaches its long-time behaviour, $x_2(t)$ still has not forgotten the trace of the initial conditions. Thus, it is the slowest degree of freedom that dictates whether the system has already reached the LLNES or not.

The previous example involved uncoupled degrees of freedom, which explains why the resulting pdf at the LLNES is expressed as the product of the pdf's for each degree of freedom independently in Eq. (II.5)—being thus a direct extension of the situation found for one-dimensional systems. Let us now consider a more involved situation, in which the potential couples the different degrees of freedom:

$$U(x_1, x_2) = \frac{1}{4}k(x_1^2 + 2x_2^2)^2, \qquad \dot{x}_1 = -bx_1(x_1^2 + 2x_2^2), \quad \dot{x}_2 = -2bx_2(x_1^2 + 2x_2^2), \quad b \equiv k/\gamma. \tag{II.6}$$

This system can also be analytically integrated. In the long-time regime, one has

$$x_1(t) \xrightarrow{\text{long } t} \pm\, (2bt)^{-1/2} \equiv \pm\, x_{\rm L}(t), \quad x_2(t) \xrightarrow{\text{long } t} x_{2,i} x_L(t)^2/x_{1,i}^2. \tag{II.7}$$

We have that $x_1(t)$ forgets the initial conditions but $x_2(t)$ never does. Nevertheless, $x_2(t)$ decays much faster than $x_1(t)$ and thus, by the time that $x_1(t)$ reaches the LLNES, $x_2(t) \ll x_1(t)$. Therefore, we conclude that

$$P_{\rm L}(x_1, x_2; t) = \frac{1}{2}\left[\delta(x_1 - x_{\rm L}(t)) + \delta(x_1 + x_{\rm L}(t))\right]\delta(x_2). \tag{II.8}$$

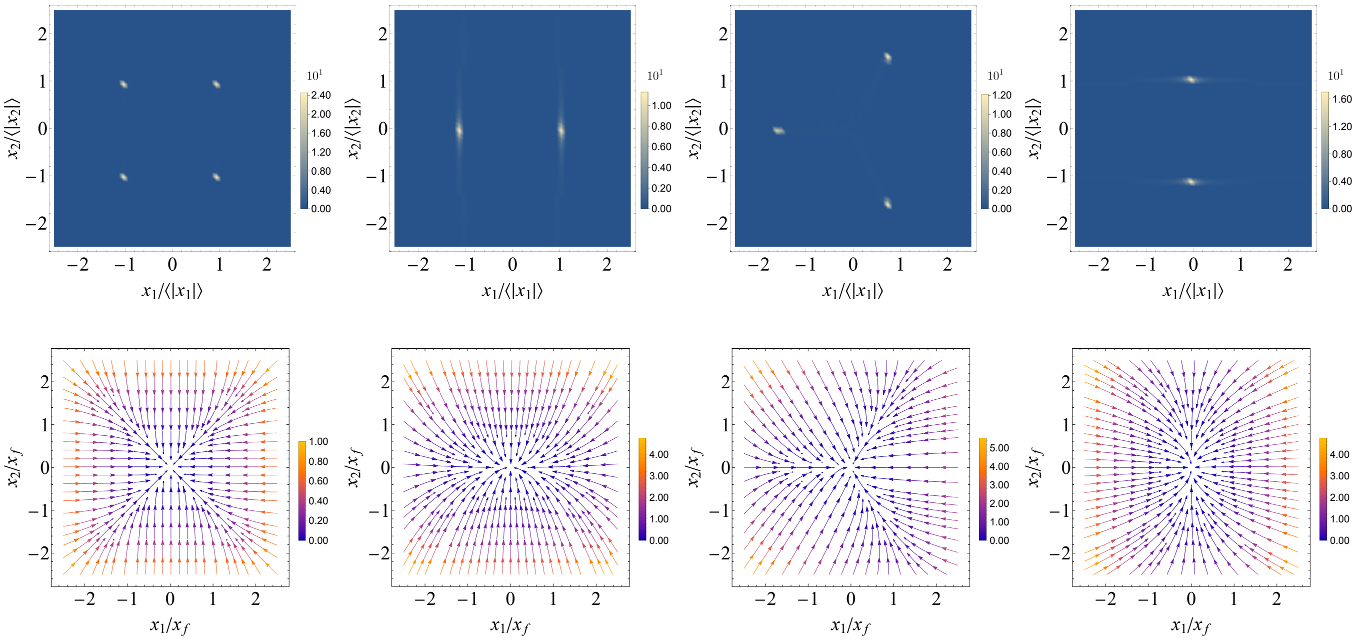


FIG. S3. Density plots of the pdf (top panels) and corresponding stream plots of the force $\boldsymbol{F} = -\nabla U$ (bottom panels). Specifically, the density plots of the pdf are presented on the $(x_1/\langle|x_1|\rangle, x_2/\langle|x_2|\rangle)$ plane, whereas the stream plots of the force are presented on the $(x_1/x_f, x_2/x_f)$ plane, where $x_f \equiv (k_B T_f/k)^{1/4}$ is a characteristic length for equilibrium at $T_f$. From left to right, the graphs correspond to the potentials in Eq. (II.3), (II.6), (II.9), and Eq. (II.11). For the latter, the pdf has been projected onto the $x_3 = 0$ plane. The density plots of the pdf are shown for a long time, once the system has reached the LLNES. To obtain the plotted pdfs, we have numerically solved the corresponding Fokker-Planck equation, including the noise term, by considering an ensemble of trajectories relaxing from very high initial temperature $T_i$ to a low enough final temperature $T_f$ such that $T_i/T_f = 10^6$.

The previous examples are quite simple, in the sense that the noiseless evolution equations can be analytically solved. The general "snowplough" picture described in Sec. II A indeed applies to these examples, as detailed below together with the remainder of the examples considered in this section. The intuitive snowplough picture can be further tested by considering a more involved potential like

$$U(\rho, \phi) = \frac{1}{4} k \rho^4 \left[2 + \cos(3\phi)\right]^2, \tag{II.9}$$

where we are employing polar coordinates, $x_1 = \rho \cos\phi$ and $x_2 = \rho \sin\phi$. This case is not analytically solvable, but the directions with slowest increase of the force are those satisfying $\cos 3\phi = -1$, i.e. $\phi = \pi/3$, $\pi$ and $5\pi/3$. We thus expect the probability to be accumulated on the vertices of an equilateral triangle, i.e. the following pdf emerges

$$P_{\mathrm{L}}(\rho, \phi; t) \propto \delta(\rho - \rho_{\mathrm{L}}(t)) \left[\delta\left(\phi - \pi/3\right) + \delta\left(\phi - \pi\right) + \delta\left(\phi - 5\pi/3\right)\right], \tag{II.10}$$

at long times, with $\rho_{\mathrm{L}}(t) \equiv (2bt)^{-1/2}$, $b \equiv k/\lambda$, being the algebraic decay solution characterising the LLNES [4].

All the cases above correspond to two-dimensional systems. Now we move to higher dimensions by looking into the three-dimensional potential

$$U(x_1, x_2, x_3) = \frac{1}{4} k (2x_1^2 + x_2^2 + 3x_3^2)^2. \tag{II.11}$$

Similarly to the potential in Eq. (II.6), this example can be solved analytically to see that $x_1(t), x_3(t) \ll x_2(t)$ by the time $x_2(t)$ reaches the LLNES, thus giving the solution

$$P_{\mathrm{L}}(x_1, x_2, x_3; t) = \frac{1}{2} \delta(x_1) \left[\delta(x_2 - x_{\mathrm{L}}(t)) + \delta(x_2 + x_{\mathrm{L}}(t))\right] \delta(x_3). \tag{II.12}$$

Following the same arguments as those employed for the potential from Eq. (II.9), the direction of the slowest increase of the force corresponds to the $x_2$-axis, i.e. $x_1 = x_3 = 0$.

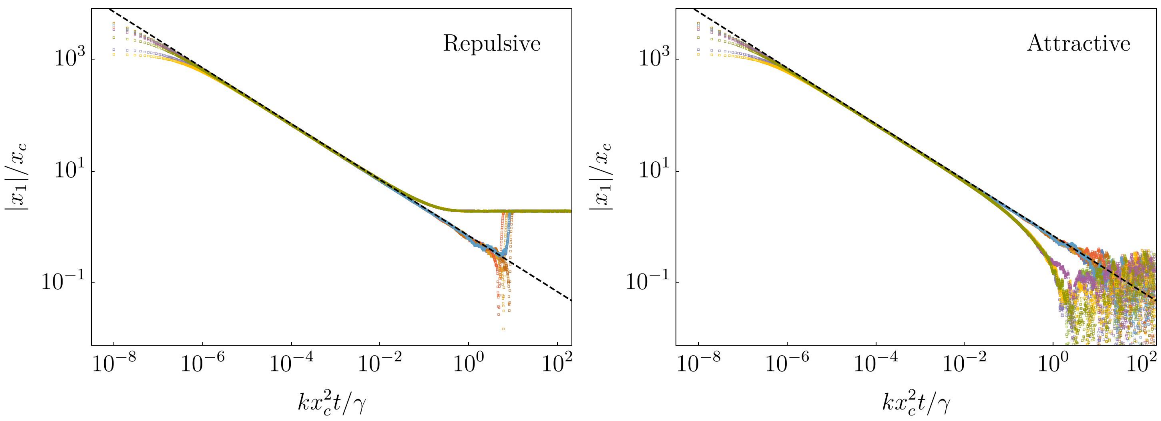


FIG. S4. LLNES for a system of two interacting particles. Specifically, we plot the modulus of the position of one of the particles, for the potential given in Eq. (II.13) with $n = 2.5$, as a function of time. The left and right panels correspond to repulsive ($c < 0$) and attractive ($c > 0$) interactions. In both panels, it is shown the relaxation from an initial equilibrium state with $k_BT_i/kx_c^4 = 10^{12}$ to a final equilibrium state with $k_BT_f/kx_c^4 = 10^{-2}$. The different coloured lines correspond to ten stochastic trajectories, corresponding to solving the Fokker-Planck equation with noise, with initial values sampled from the equilibrium distribution at $T_i$. The black, dashed line corresponds to the solution at the LLNES, given by Eq. (II.2).

Fig. S3 shows the density plots of the pdf for each of the potentials presented in this section (top panels), together with plots showing the stream lines of the corresponding "force" (bottom panels). It is clearly observed that the directions over which the Dirac-delta peaks emerge are those for which the force increases the slowest. These stream plots neatly illustrate that each of these directions have its own basin of attraction, thus supporting—on an intuitive basis—the "snowplough" picture described before in Sec. II A. The snowplough sweeps the snow (probability weight) on the directions of fastest variation of the force and accumulates it on the slowest ones.

### D. Interacting degrees of freedom

So far, in order to highlight the role of the non-harmonic confining potential in the emergence of the LLNES, we have considered non-interacting systems. We now show that the LLNES is resilient to the inclusion of interactions.

Let us consider the following potential for two degrees of freedom,

$$U(x_1, x_2) = \frac{1}{4}k(x_1^4 + x_2^4) + \frac{1}{n}c\,|x_1 - x_2|^n, \tag{II.13}$$

i.e. two particles, with positions $x_1$ and $x_2$, which are both confined in the same one-dimensional quartic potential while interacting with a potential that depends on the relative distance between them. The $c$ constant determines whether the interaction is attractive ($c > 0$) or repulsive ($c < 0$), while $n$ quantifies the strength of the interaction. The system is once more submitted to a quench, the initial temperature being much larger than the final one.

First, we consider the repulsive case. Here, we restrict to $n < n_{\text{crit}} = 4$: otherwise, the interaction potential becomes so strong that the particles are no longer confined and the system never reaches equilibrium. For sufficiently high temperatures, the system initially does not feel the effect of the interactions and thus relaxes as in the non-interacting case. The repulsive interaction induces an additional characteristic length $x_c \equiv (|c|/k)^{1/(4-n)}$ that becomes significant only when the system approaches the bottom of the potential.

In the attractive case, the resulting potential is confining for all values of $n$. The effect of interactions now entails the emergence of a new characteristic timescale corresponding to *sticking*: particles tend to move together, i.e. relax along the line $x_1 = x_2$. On the one hand, if $n > n_{\text{crit}} = 4$, the particles rapidly stick and afterwards relax together towards the LLNES. On the other hand, if $n < n_{\text{crit}} = 4$, interactions are subdominant with respect to the confining potential. Thus, the relaxation is again similar to that of the non-interacting case initially, with the interaction becoming relevant only close to the bottom of the potential.

Figure S4 shows the relaxation for one of the particles, when the system is quenched from a sufficiently high temperature. On the left (right) panel, the repulsive (attractive) case is shown. As commented above, repulsive interactions introduce the new characteristic length $x_c$, related to that of mechanical equilibrium of the system. In this sense, the role of repulsive interactions is similar to that of multistability, note the analogy with the time evolution displayed in Fig. S2. For attractive interactions, those trajectories for which the sign of the initial conditions $x_{1,i}$ and

$x_{2,i}$ are equal continue together over the LLNES until noise becomes relevant; those trajectories for which the sign of the initial conditions $x_{1,i}$ and $x_{2,i}$ are different deviate from it to switch to the other side of the potential and facilitate the sticking of the two particles. A part of this switching behaviour is still noiseless and resembles the extension to longer times of the LLNES in Eq. (17) of the main text.

Note that the physical systems analysed in this supplemental material have been motivated by overdamped systems in confining potentials, and thus we have interpreted the Markovian process $\boldsymbol{r} = \{x_1, x_2, ..., x_d\}$ as the position of one Brownian particle in a $d$-dimensional confining potential—or several Brownian particles moving in lower dimensions, e.g. $d$ of them. However, the results above apply to any physical system whose degrees of freedom—not necessarily position coordinates—are described in terms of non-linear Langevin equations.

### E. A non-linear fluid of interacting particles

Now we consider a non-linear fluid of interacting particles, which further broadens the scope of application of our ideas. Specifically, we consider the isotropic fluid with non-linear drag force investigated in Refs. [5–7]: a system of Brownian particles with number density $n$, modelled as $d$-dimensional hard spheres of diameter $\sigma$ and mass $m$, is suspended in a background fluid at equilibrium at temperature $T_f$. Its one-particle velocity pdf $P(\boldsymbol{v}, t)$ obeys the Boltzmann-Fokker-Planck equation (18) of the main text. The Boltzmann collision term accounts for—possibly inelastic—two-particle collisions between the Brownian particles, which cannot be considered in a pure Fokker-Planck (or Langevin) description [8].

It is useful to introduce the kinetic temperature $T_{\text{kin}}(t)$ as in the main text, the associated thermal velocity $v_{\text{th}}(t)$, and scaled variables as

$$v_{\text{th}}(t) = \sqrt{\frac{2k_B T_{\text{kin}}(t)}{m}}, \quad \phi(\boldsymbol{c}, t) \equiv v_{\text{th}}^d(t)\, P(\boldsymbol{v}, t), \quad \boldsymbol{c} \equiv \frac{\boldsymbol{v}}{v_{\text{th}}(t)}, \quad \theta(t) = \frac{T_{\text{kin}}(t)}{T_f}, \quad t^* \equiv \zeta_0 t. \tag{II.14}$$

We carry out the analysis for the family of non-linear drag forces introduced in the main text: the drag coefficient is written as $\zeta(v) = \zeta_0 \zeta^*(v/v_{\text{th},f})$, where $\zeta_0 \equiv \zeta(v = 0)$, and $v_{\text{th},f}$ is the thermal velocity at $T_f$, i.e. $v_{\text{th},f} \equiv \sqrt{2k_B T_f/m}$. The resulting evolution equation for the scaled velocity distribution function $\phi(\boldsymbol{c}, t)$ reads [5, 6]

$$\partial_{t^*}\phi = \nabla_{\boldsymbol{c}} \cdot \left\{ \left[ \frac{\dot\theta}{2\theta}\boldsymbol{c} + \zeta^*(\sqrt{\theta}c) \left( \boldsymbol{c} + \frac{1}{2\theta}\nabla_{\boldsymbol{c}} \right) \right] \phi \right\} + \xi^{-1}\theta^{1/2} J^*[\phi, \phi], \tag{II.15}$$

Here, $\dot\theta \equiv d\theta/dt^*$, $\nu_s \equiv n\sigma^{d-1}\sqrt{2k_B T_f/m}$ is the (equilibrium) collision frequency at temperature $T_f$, $J^*[\phi, \phi]$ stands for the dimensionless collision operator, and $\xi \equiv \zeta_0/\nu_s$ accounts for the relative significance of collisions with respect to the non-linear drag. For $\xi \gg 1$, collisions occur over a timescale that is much longer than that of the drag force, in this case collisions are thus negligible (the Fokker-Planck term suffices to drive the system to equilibrium at $T_f$), whereas for $\xi = O(1)$ collisions and the drag force act over the same timescale. If collisions are elastic, the evolution equation for the scaled temperature is [5, 6]

$$\dot\theta = -\frac{4}{d}\theta \left\langle c^2 \zeta^*(c\sqrt{\theta}) \right\rangle + \frac{2}{d} \left( \left\langle c \frac{\partial \zeta^*(c\sqrt{\theta})}{\partial c} \right\rangle + d \left\langle \zeta^*(c\sqrt{\theta}) \right\rangle \right). \tag{II.16}$$

Now we consider the family of drag coefficients introduced in the main text, for which $\zeta^*(u) \sim \gamma u^n$ for large $u$, with $\gamma$ being a constant measuring the strength of the nonlinearity. The different terms in Eq. (II.15) scale as distinct powers of the dimensionless temperature $\theta$: for sufficiently high initial temperatures, $\theta \gg 1$, it is the most diverging contribution in $\theta$ that rules the relaxation. The dominant terms stemming form the non-linearity are $O(\theta^{n/2})$ while the one accounting for the collisions is $O(\theta^{1/2})$, so collisions become negligible as long as $n > 1$. Therefore, the system will tend naturally towards the LLNES for $n > 1$, and remain over it as long as the temperature keeps being high enough. Following a reasoning completely similar to that in Sec. I C 1, it is shown that there exists an asymptotic solution of the Dirac-delta form, $\phi_{\text{L}}(\boldsymbol{c}) \propto \delta(c - \sqrt{d/2})$, which is centred around $c = \sqrt{d/2}$ due to the particular choice of $\boldsymbol{c}$ in Eq.(II.14)—such that $\langle c^2 \rangle = d/2$. In this time regime, the dominant term in the evolution equation of the scaled temperature (II.16) is

$$\dot\theta \sim -(4\gamma/d)\, \theta^{(n+2)/2} M_{n+2}, \tag{II.17}$$

where $M_m \equiv \langle c^m \rangle$. Since all the moments $M_m$ become time-independent over the LLNES, $\dot\theta \propto -\theta^{(n+2)/2}$ which implies a non-exponential algebraic decay. Note that inelastic collisions would introduce an additional term, proportional to $\theta^{3/2}$ [9], on the rhs of Eq. (II.16). Therefore, this term is negligible for $\theta \gg 1$ as long as $n > 1$.

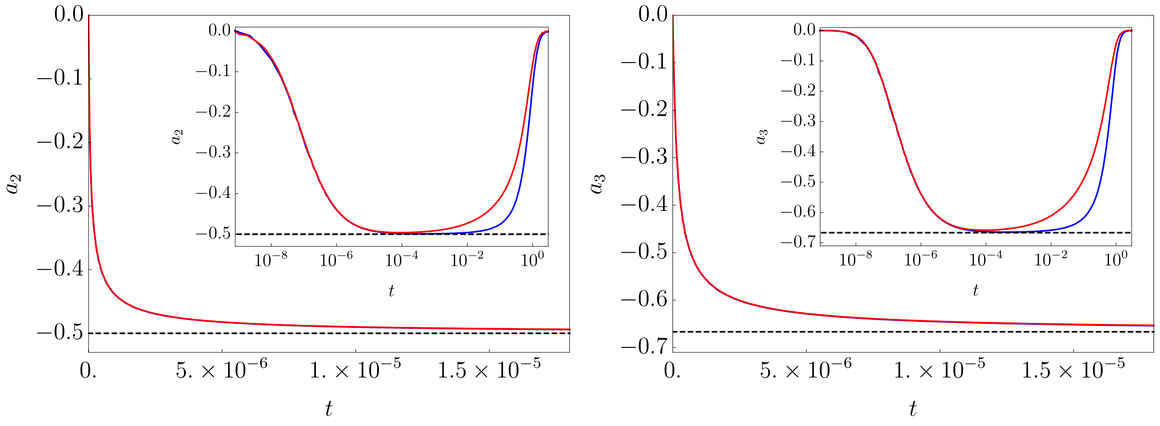


FIG. S5. Time evolution of the excess kurtosis $a_2$ (left) and the sixth cumulant $a_3$ (right). The main panels show their relaxation towards the LLNES, for $n = 2$, $\gamma = 0.1$, $d = 2$, $N = 10^6$ particles and two values of $\xi$, $\xi = 1$ (red) and $\xi = 10$ (blue). The system relaxes from an initial equilibrium distribution with temperature $T_i$ to a final one $T_f$, such that $\theta_i = T_i/T_f = 10^7$. Black, dashed lines correspond to the asymptotic values attained at the LLNES, which are given by Eq. (II.19). The relaxation towards the LLNES is independent of the value of $\xi$, i.e. of the relevance of collisions. Both insets show the time evolution in logarithmic scale, in which it is observed that the system eventually returns to equilibrium—at which both $a_2$ and $a_3$ vanish– for longer times. The LLNES lasts longer for $\xi = 10$ than for $\xi = 1$ because in the former case collisions, which accelerate thermalisation, come into play for longer times.

In order to visualise the tendency to the LLNES and its being a far-from-equilibrium state, it is illustrative to consider the cumulants of the pdf in the typical Sonine expansion employed in kinetic theory [9, 10], which are zero for the equilibrium Maxwellian pdf. In particular, here we employ the first two of them: the fourth cumulant (excess kurtosis) $a_2$ and the sixth cumulant $a_3$,

$$a_2 \equiv -1 + \frac{4}{d(d+2)} M_4, \quad a_3 \equiv 1 + 3a_2 - \frac{8}{d(d+2)(d+4)} M_6. \tag{II.18}$$

Over the LLNES, these cumulants have the values

$$a_{2,\mathrm{L}} \equiv -\frac{2}{d+2}, \quad a_{3,\mathrm{L}} \equiv -\frac{16}{(d+2)(d+4)}. \tag{II.19}$$

Fig. S5 presents the time evolution of both cumulants. Regardless of collisions, which try to thermalise the system towards equilibrium, both cumulants tend to their corresponding LLNES values within an intermediate timescale. It is only for longer times that collisions and noise come into play and make the system go to equilibrium at the final temperature $T_f$, at which both cumulants vanish—as shown in the insets.

## ACKNOWLEDGMENTS

A. Patrón, B. Sánchez-Rey and A. Prados acknowledge financial support from Grant No. PID2021-122588NB-I00 funded by MCIN/AEI/ 10.13039 /501100011033/ and by "ERDF A way of making Europe". All the authors acknowledge financial support from Grant No. ProyExcel_00796 funded by Junta de Andalucía's PAIDI 2020 programme. A. Patrón acknowledges support from the FPU programme through Grant FPU2019-4110, and also additional support from the FPU programe through Grant EST22/00346, which funded his research stay at Univ. Paris-Saclay during autumn 2022. A. Prados also acknowledges the hospitality of LPTMS, which funded his stay at Univ. Paris-Saclay in June 2022.

[1] We use quotation marks here because $r$ may not be a distance.

[2] If the first and/or second moments of $\phi_{\mathrm{st}}$ diverge, it can be shown that, depending on the value of $n$ and the choice of $P_i^*$, the standard deviation of $\phi_{\mathrm{st}}$ diverges either logarithmically or algebraically as $r_{\mathrm{L}}^*(t) \to 0$. In any case, the standard deviation for $r^*$, $\sigma_{r^*}^*(t)$, decays always in such a way that $\sigma_{r^*}^*(t)/\langle r^* \rangle(t) \to 0$.

[3] M. Loève, *Probability Theory I*, Vol. 1 (Springer New York, 1997).
[4] Over the direction such that $\cos 3\phi = -1$, $\dot{\rho} = -b\rho^3$, $b \equiv k/\gamma$, which in the long-time limit gives once more $\rho \sim (2bt)^{-1/2}$.
[5] A. Santos and A. Prados, Mpemba effect in molecular gases under nonlinear drag, Physics of Fluids **32**, 072010 (2020).
[6] A. Patrón, B. Sánchez-Rey, and A. Prados, Strong nonexponential relaxation and memory effects in a fluid with nonlinear drag, Physical Review E **104**, 064127 (2021).
[7] A. Megías, A. Santos, and A. Prados, Thermal versus entropic Mpemba effect in molecular gases with nonlinear drag, Physical Review E **105**, 054140 (2022).
[8] Note that collisions may be inelastic.
[9] T. Pöschel and S. Luding, eds., *Granular Gases*, Lecture Notes in Physics 564 (Springer-Verlag Berlin Heidelberg, 2001).
[10] S. Chapman, T. Cowling, D. Burnett, and C. Cercignani, *The Mathematical Theory of Non-uniform Gases: An Account of the Kinetic Theory of Viscosity, Thermal Conduction and Diffusion in Gases*, Cambridge Mathematical Library (Cambridge University Press, 1990).
